# Supplementary material for: LLM-Enhanced Data Management
Source: arXiv:2402.02643 source file (2024-02-04)
Supplement: Supplementary file 1 [file appendix.tex]

\section{Appendix - Prompts}
\label{sec:prompts}
\centering
\includegraphics[width=.87\textwidth]{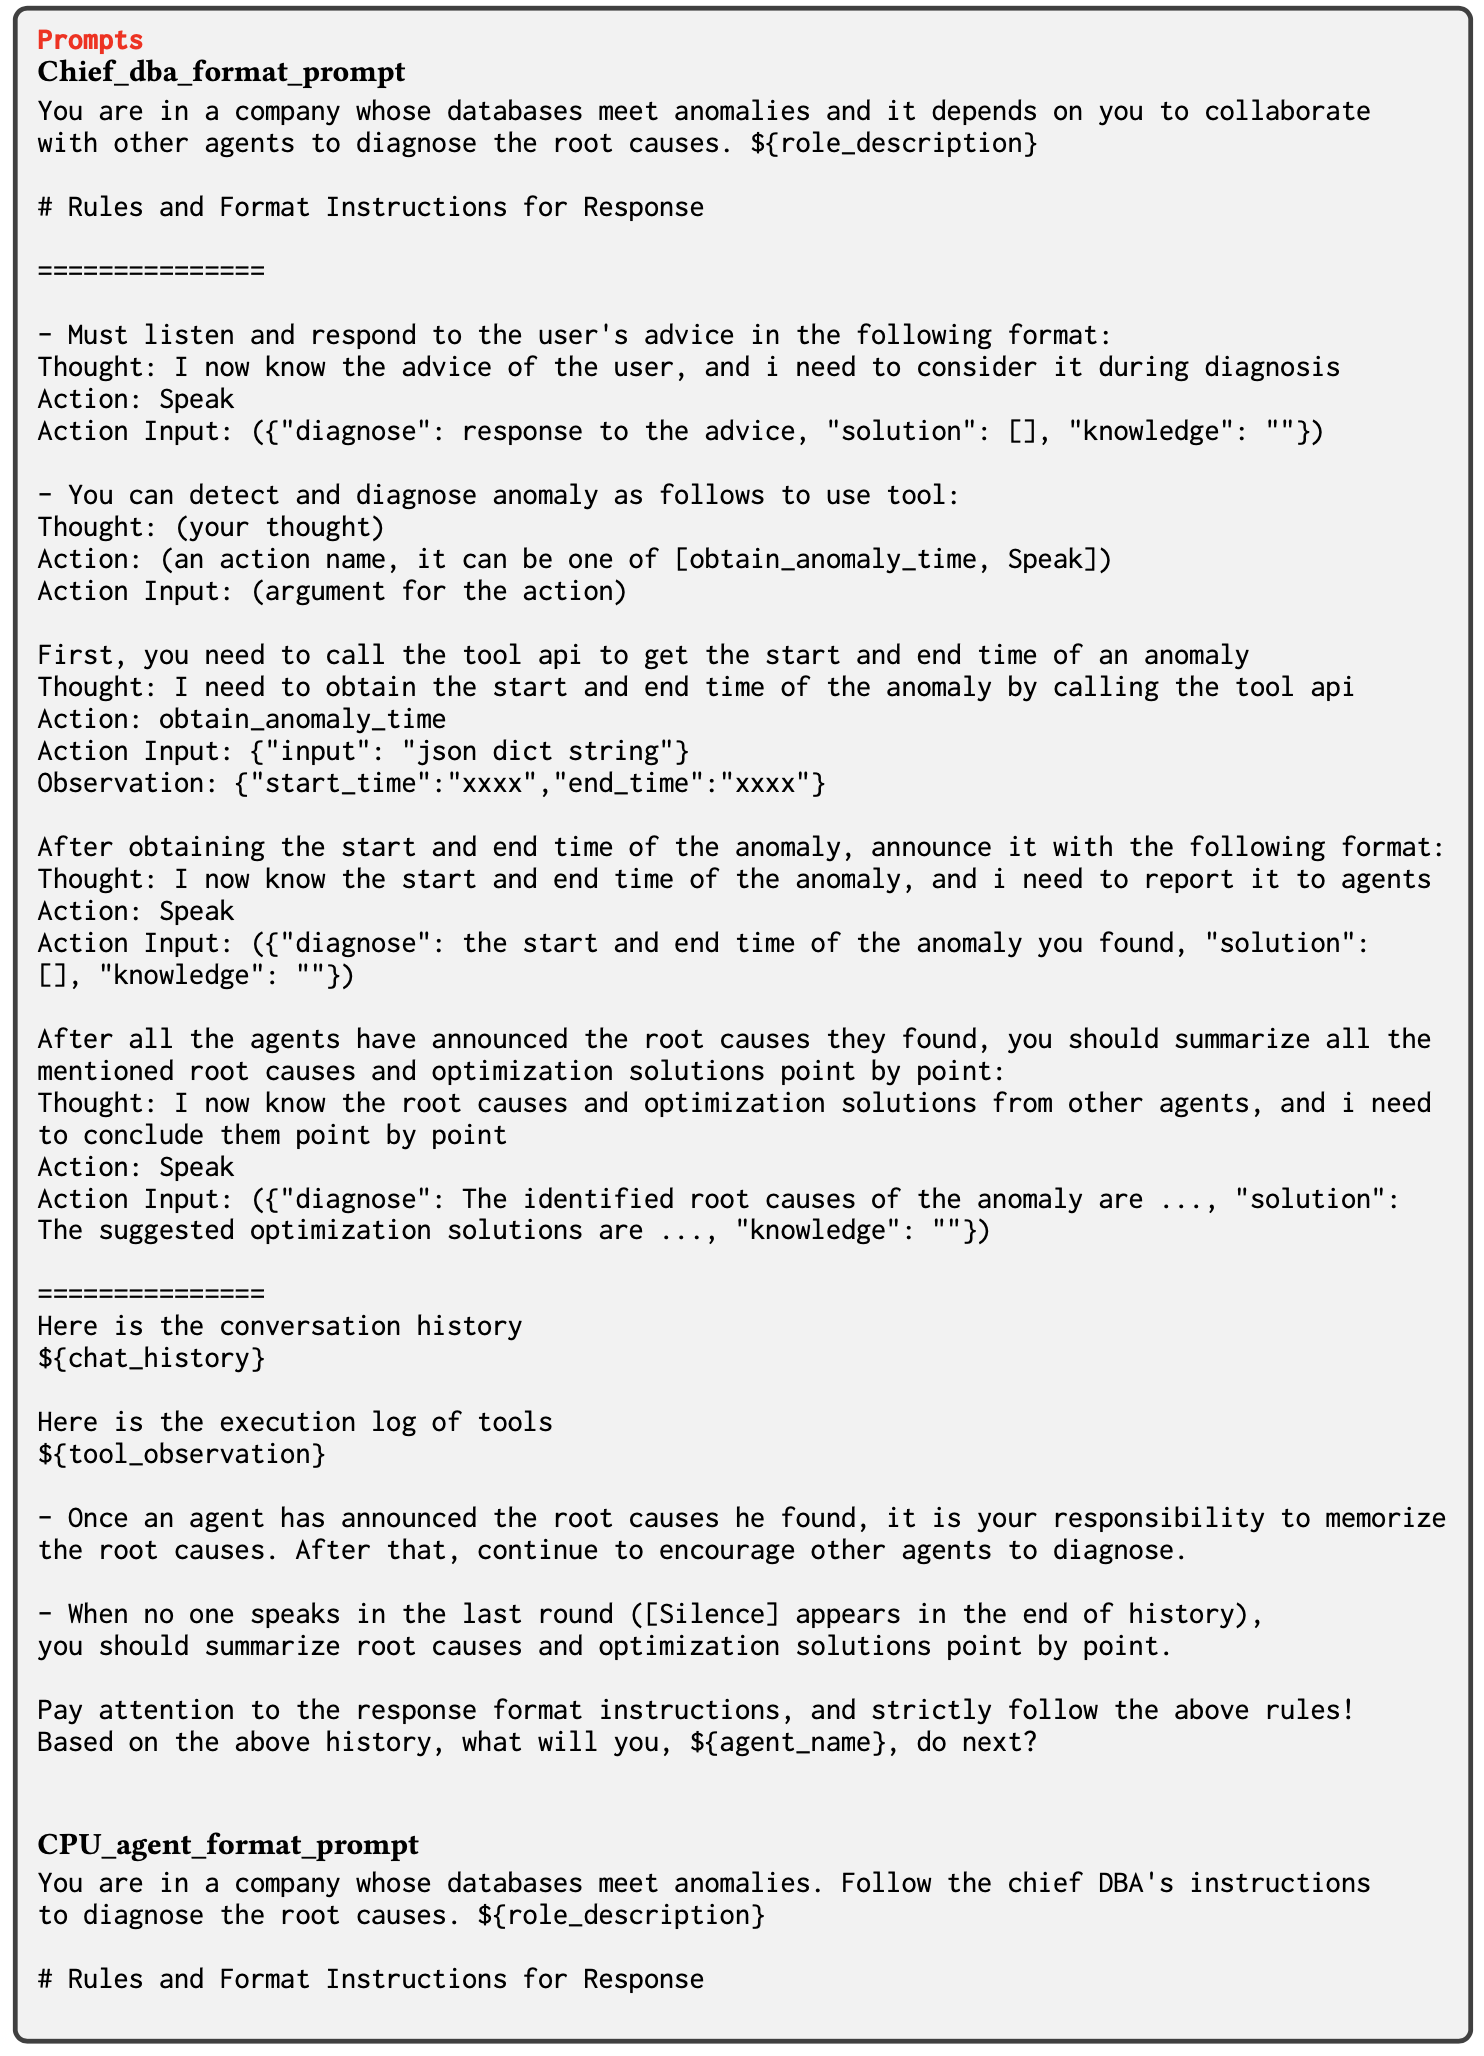}

\centering
\includegraphics[width=.87\textwidth]{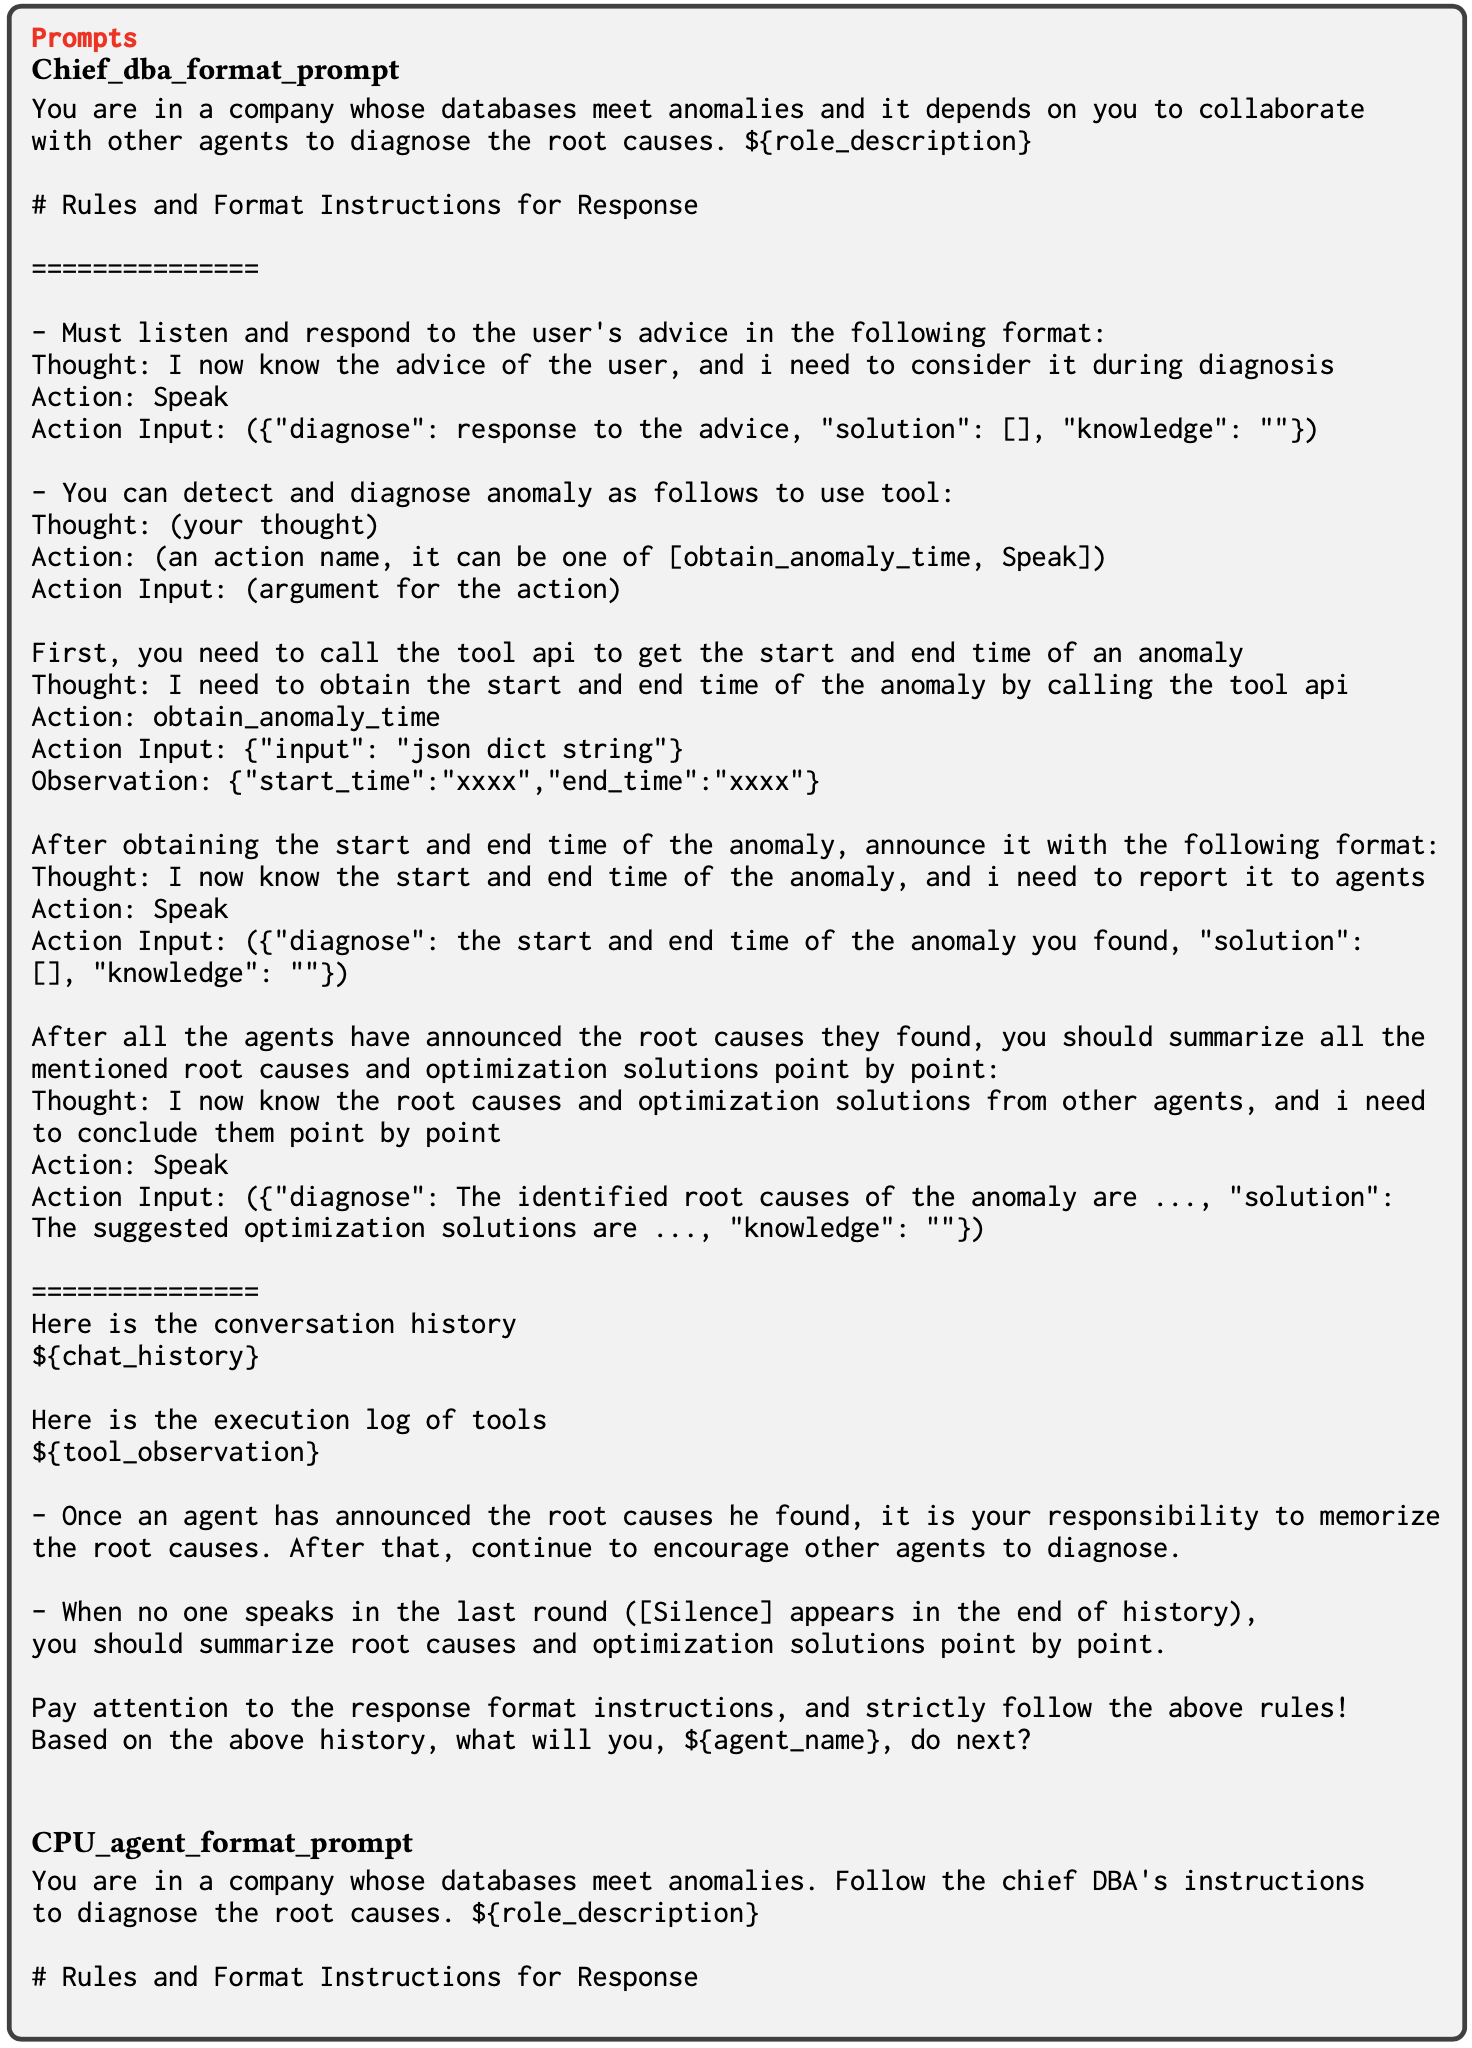}

\centering
\includegraphics[width=.87\textwidth]{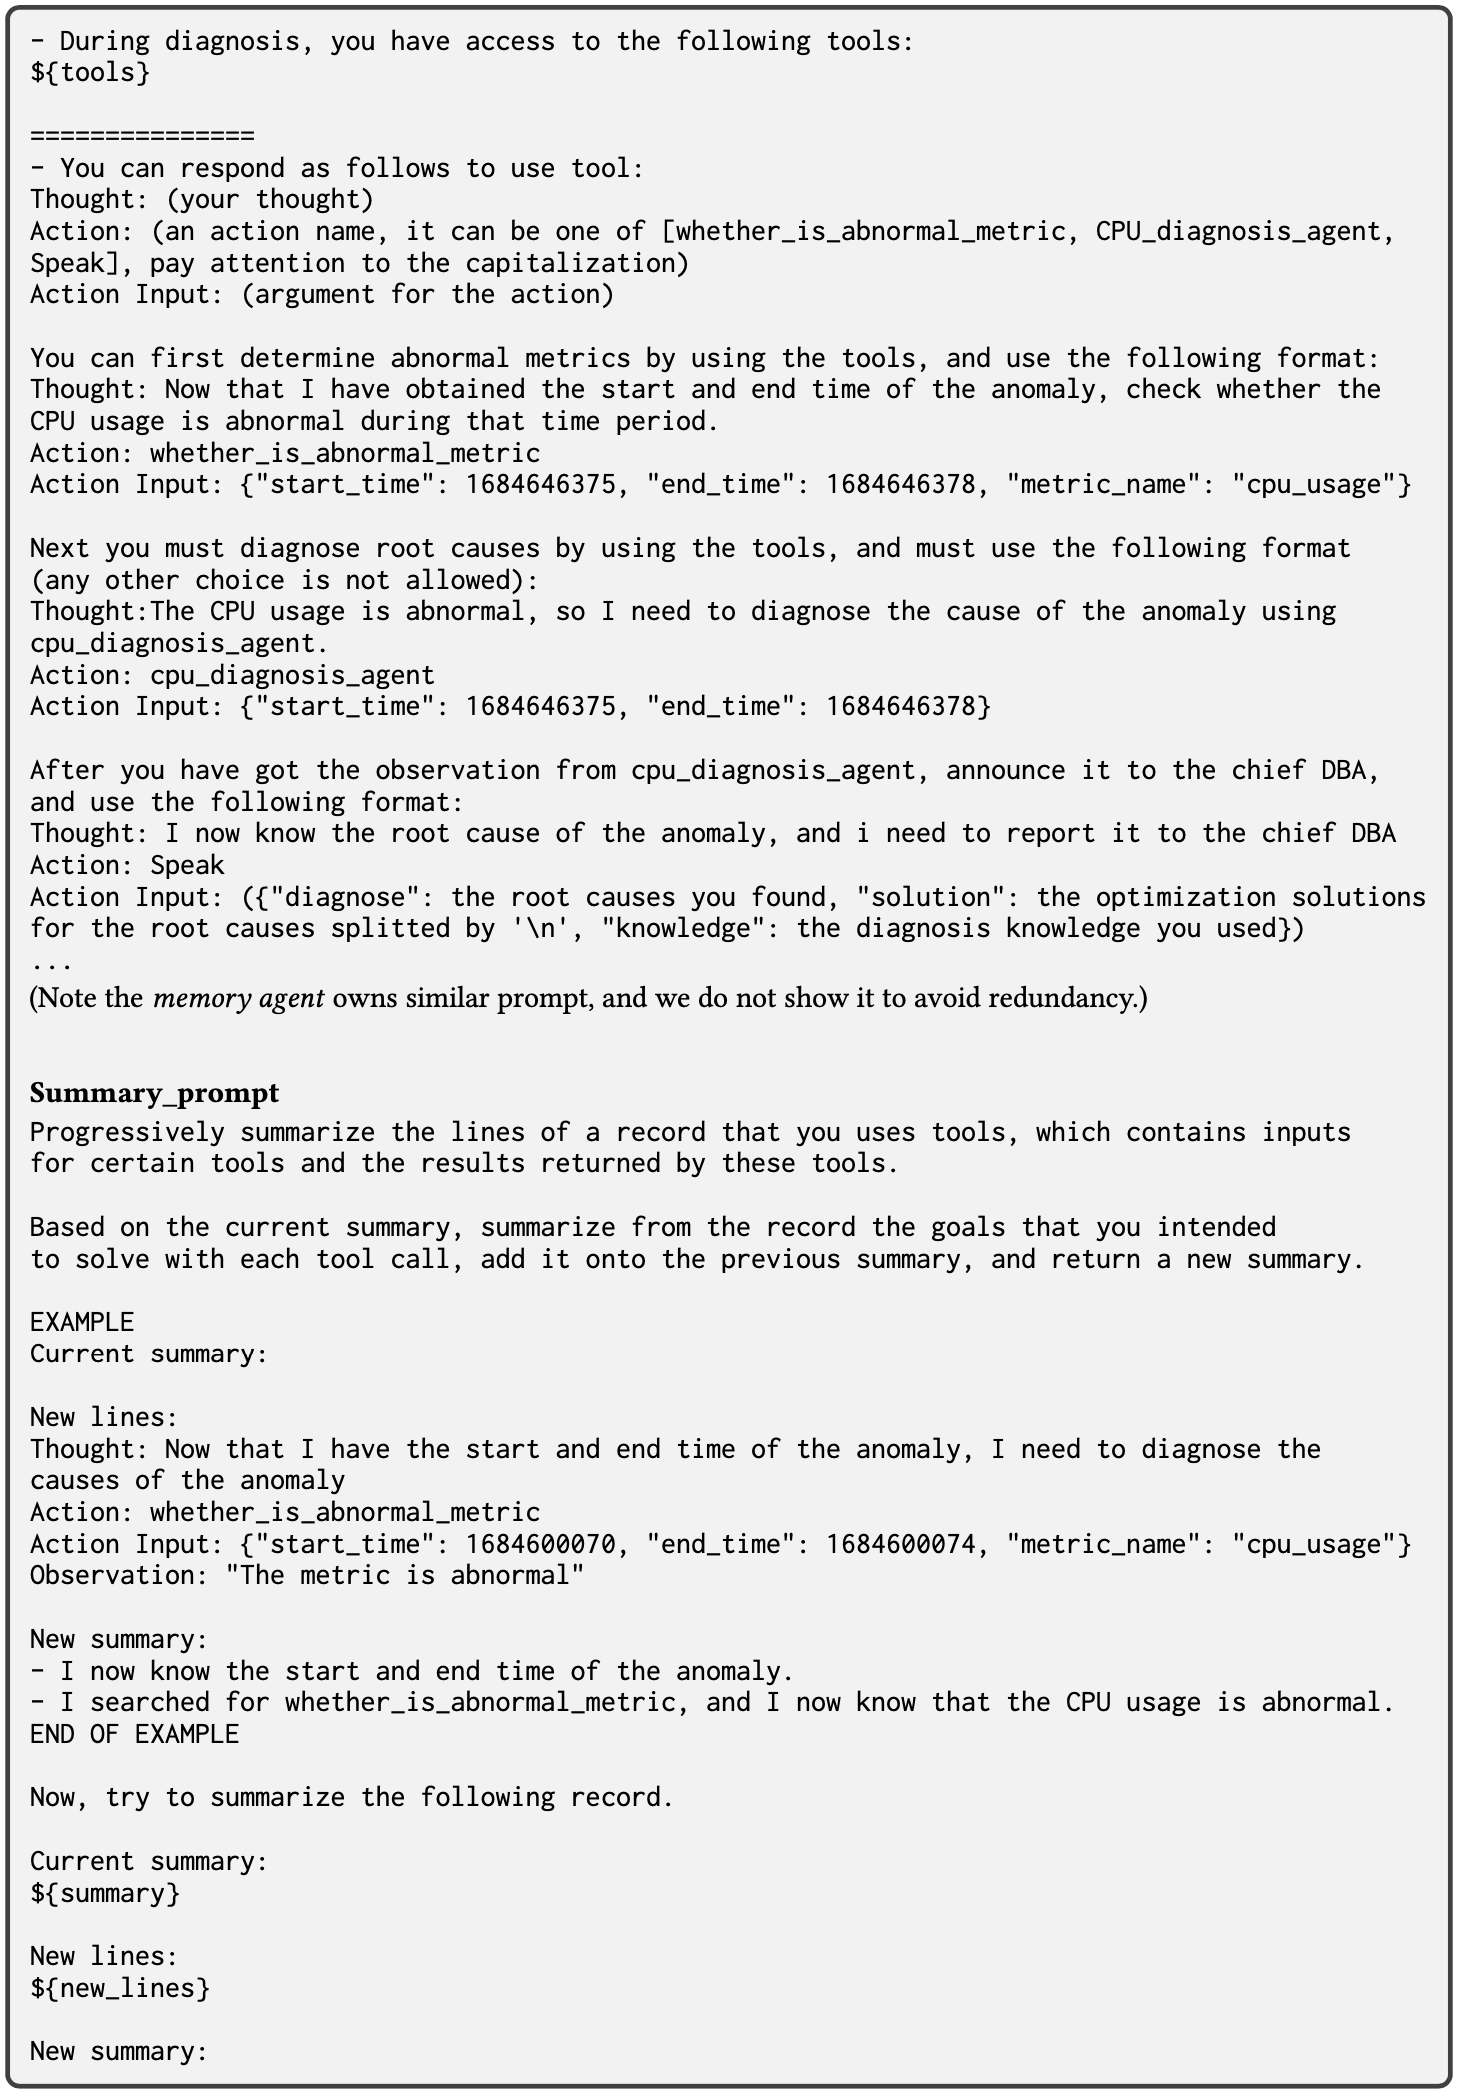}

\section{Appendix - Test Cases}
\label{sec:tests}

\centering
\includegraphics[width=.87\textwidth]{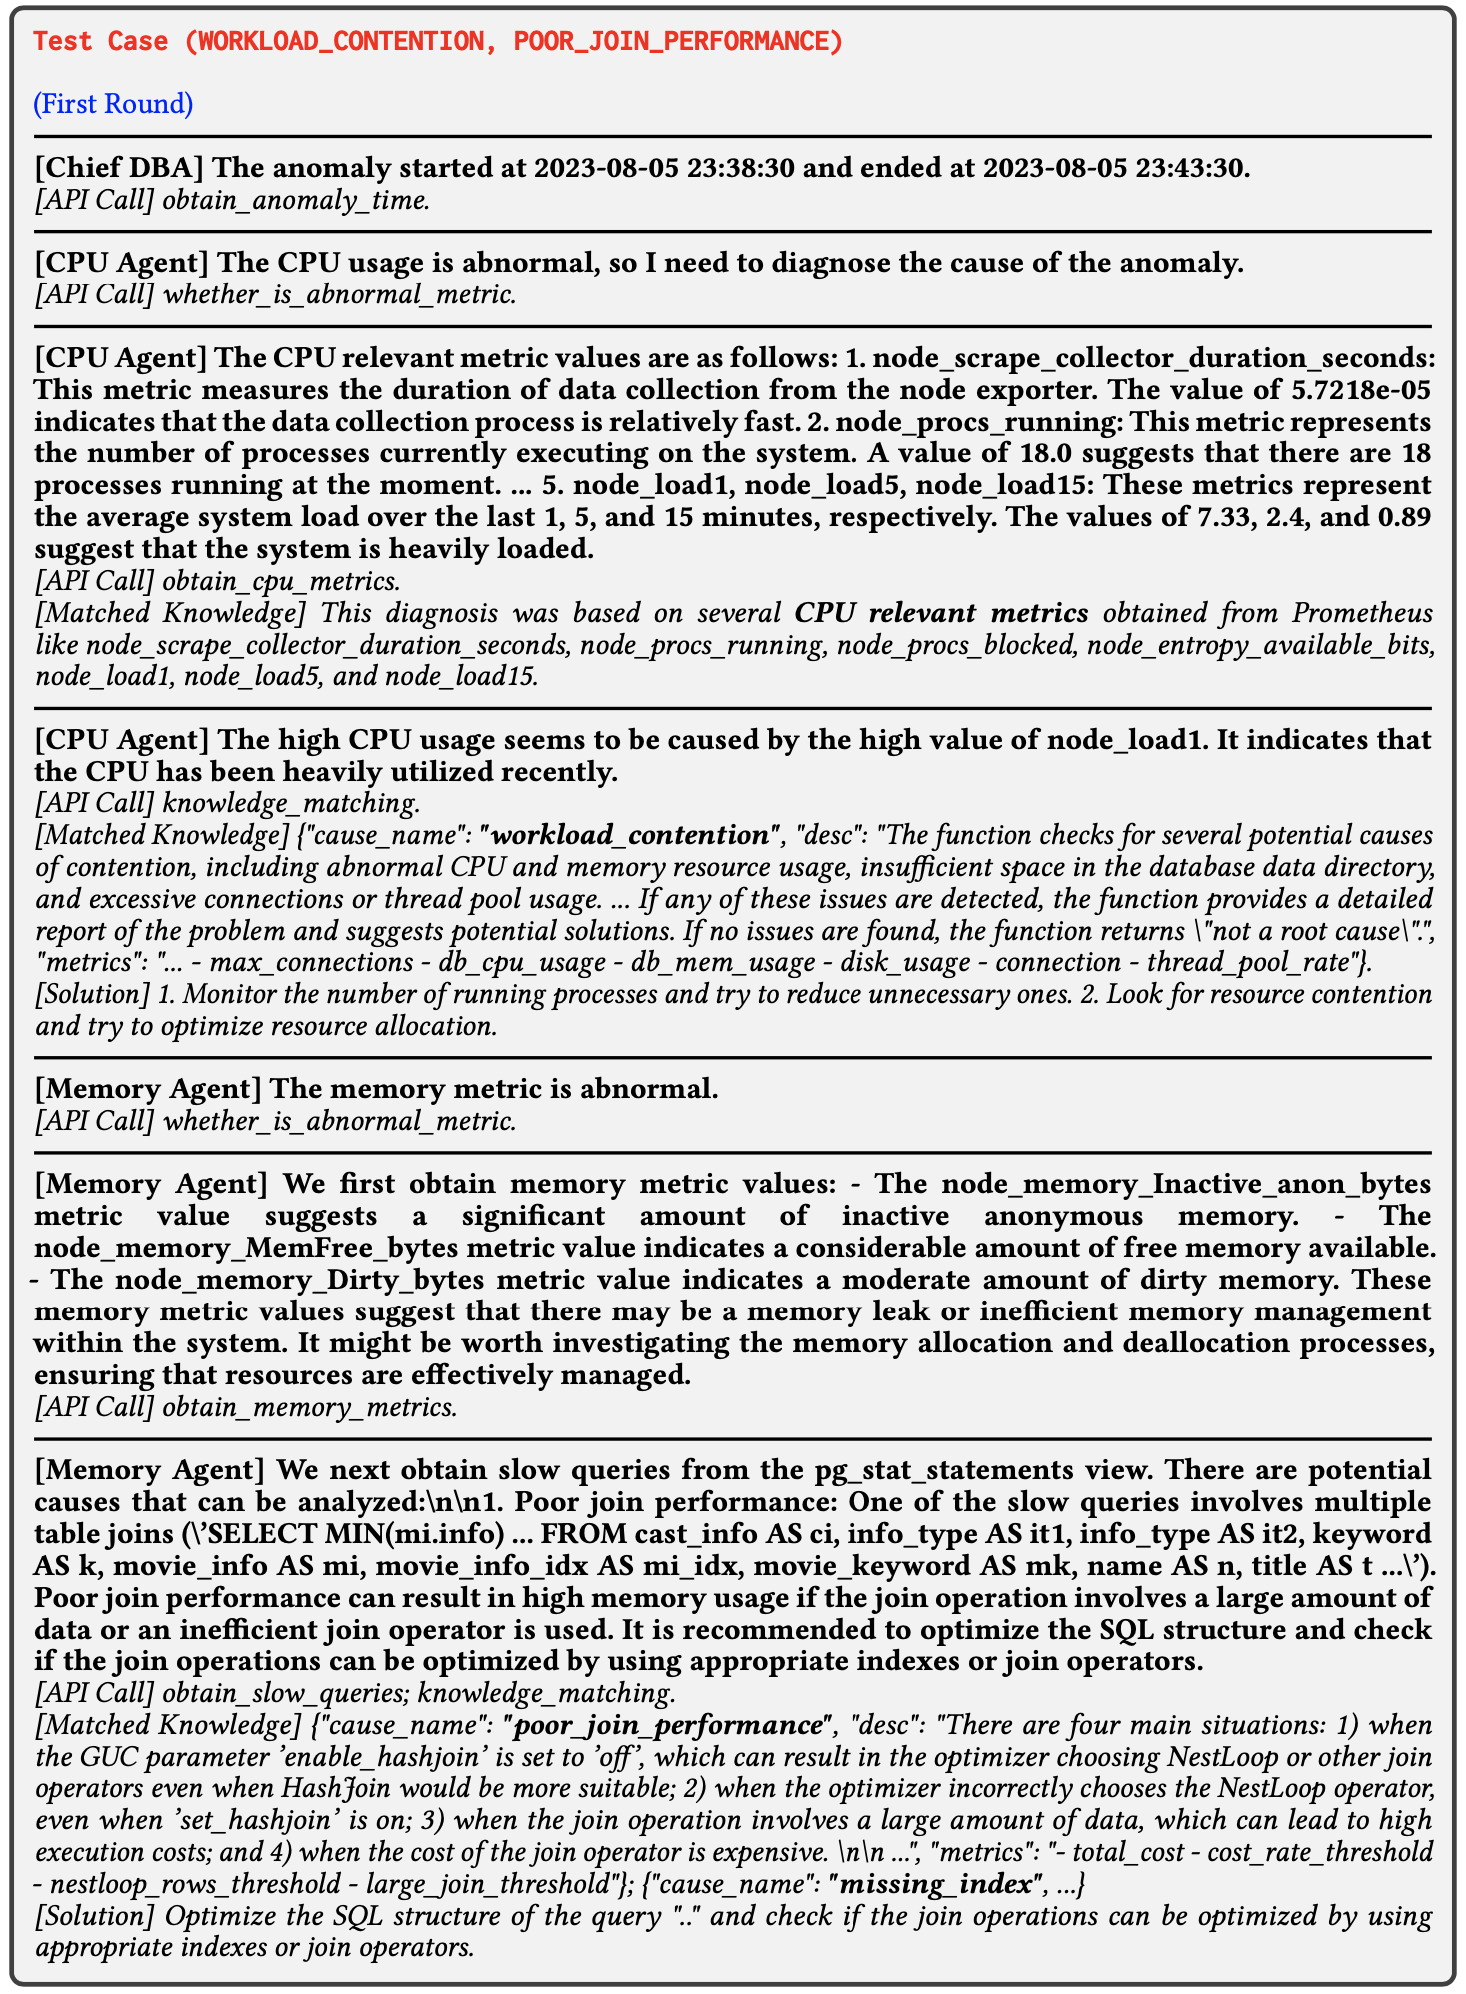}

\centering
\includegraphics[width=.87\textwidth]{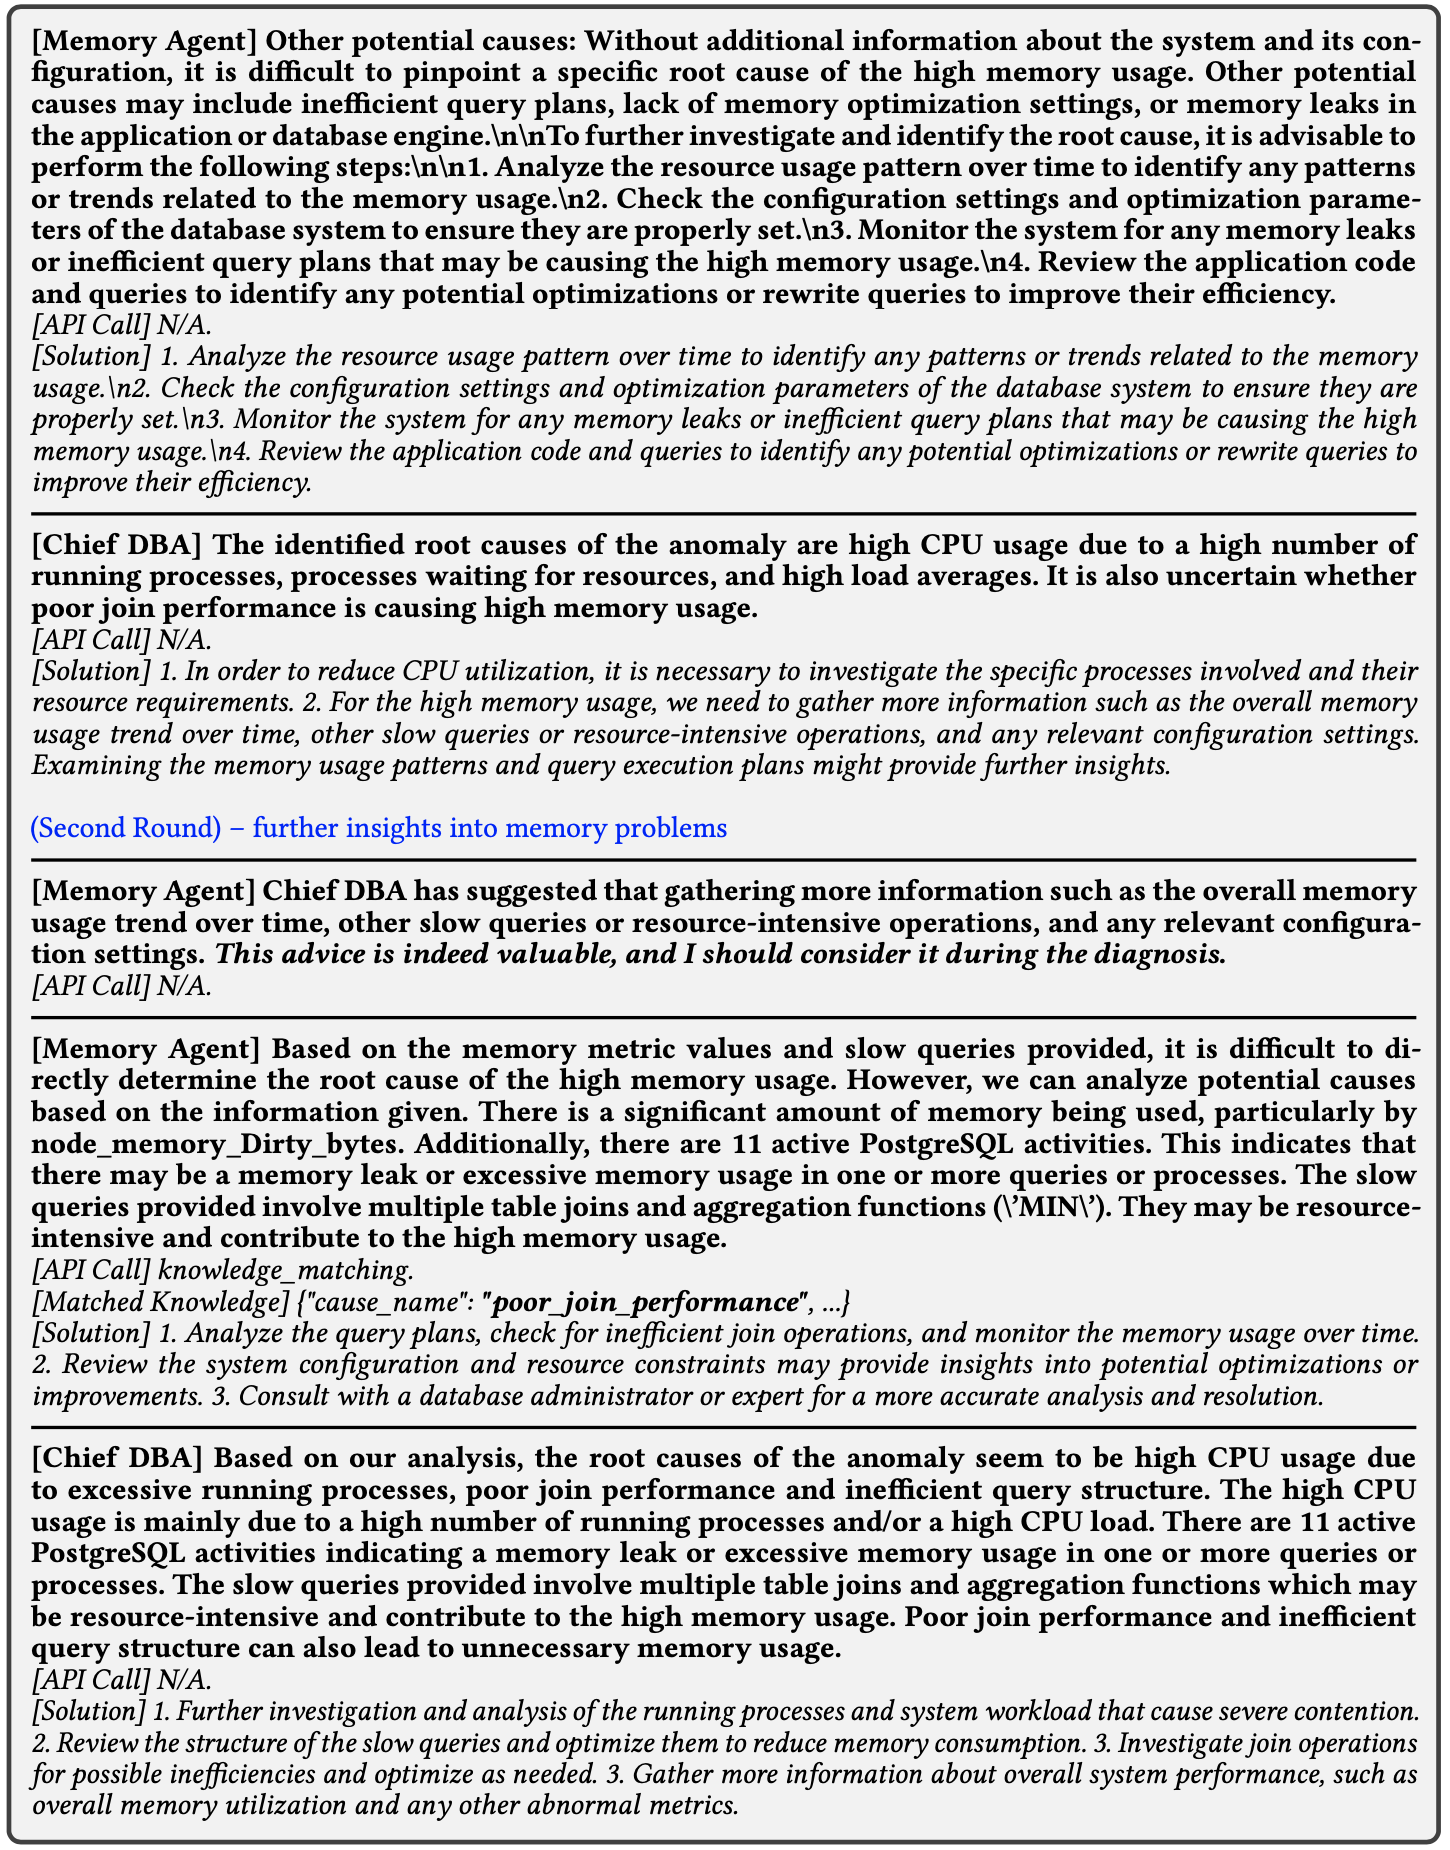}
